# Supplementary material for: Hosting Industry Centralization and Consolidation
Source: arXiv:2109.01187 source file (2022-01-25)
Supplement: Supplementary file 1 [file appendix.tex]

\appendix

\section{Extra graphs and data}

\autoref{tab:listTLDs} shows the list of TLDs we evaluted in this study, and their country (for ccTLDs).

\begin{table}
\centering
 \begin{tabular}{ccc}
 \textbf{TLD}& \textbf{Country}& \textbf{Type}\\
 \dns{.at}        & Austria                  & ccTLD \\
 \dns{.ca}        & Canada                   & ccTLD \\
 \dns{.ch}        & Switzerland              & ccTLD \\
 \dns{.co}        & Colombia                 & ccTLD \\
 \dns{.dk}        & Denmark                  & ccTLD \\
 \dns{.ee}        & Estonia                  & ccTLD \\
 \dns{.fi}        & Finland                  & ccTLD \\
 \dns{.gt}        & Guatemala                & ccTLD \\
 \dns{.li}        & Liechtenstein            & ccTLD \\
 \dns{.na}        & Namibia                  & ccTLD \\
 \dns{.nl}        & The Netherlands          & ccTLD \\
 \dns{.nu}        & Niue                     & ccTLD \\
 \dns{.ru}        & Russian Federation       & ccTLD \\
 \dns{$\mathbf{.p\phi}$} & Russian Federation       & ccTLD   \\
 \dns{.se}        & Sweden                   & ccTLD \\
 \dns{.us}        & United States of America & ccTLD \\
 \dns{.com}       & International                     & gTLD  \\
 \dns{.net}       & International                      & gTLD  \\
 \dns{.org}       & International                      & gTLD 
 \end{tabular}
 \caption{List of TLDs evaluted in the paper}
 \label{tab:listTLDs}
\end{table}

\autoref{tab:listtASes} shows the list of ASes we see in the five years for all TLDs combined. 

\begin{table}
    \centering
    \small
    \begin{tabular}{ccc}
        \textbf{AS Number}& \textbf{AS Name}& \textbf{Country}\\
        6724   & Strato AG                  & DE \\
        8560   & 1\&1 IONOS SE              & DE \\
        13335  & Cloudflare, Inc.           & US \\
        14618  & Amazon.com, Inc.           & US \\
        16509  & Amazon.com, Inc.           & US \\
        15169  & Google LLC                 & US \\
        16276  & OVH SAS                    & FR \\
        20773  & Host Europe GmbH           & DE \\
        20857  & eTOP sp. z o.o.            & PL \\
        22612  & Namecheap, Inc.            & US \\
        26496  & GoDaddy.com, LLC           & US \\
        29873                               & The Endurance International Group, Inc. & US                                \\
        34011  & Yahoo! UK Services Limited & GB \\
        40034  & GearHost, Inc.             & US \\
        43081  & WebConnect                 & US \\
        46606  & Unified Layer              & US \\
        48635  & PCextreme B.V.             & NL \\
        51468  & One.com A/S                & DK \\
        51696  & Antagonist B.V.            & NL \\
        53831  & Squarespace, Inc.          & US \\
        58182  & Wix.com Ltd.               & IL \\
        59980  & Mijndomein Hosting B.V.    & NL \\
        63949  & Linode, LLC                & US \\
        91232   & TimeWeb Ltd.               & RU \\
        197695                              & Domain names registrar REG.RU, Ltd      & RU                                \\
        197902 & Hostnet B.V.               & NL 
    \end{tabular}
    \caption{List of ASes and their names and countries}
    \label{tab:listtASes}
\end{table}

\section{IPv6 dataset and results}
\label{sec:ipv6-results}

\autoref{tab:top5-2021-ipv6} shows the top 5 hosting ASes for IPv6 in 2021.

% \begin{table}
%     \centering
%     \begin{tabular}{ccccc}
%         \textbf{\#}& \textbf{ASN}& \textbf{Country}& \textbf{Domains }& \textbf{Ratio}\\ 
%         1  & 13335-GoDaddy&US&	5.7M&26\%\\
%         2 & 16509-AWS&	US&2.4M&11.3\% \\ 
%         3&8560-1\&1& DE& 	2.4M& 11.1\% \\ 
%         4&15169-Google&US&	2.0M& 9.2\%\\ 
%         5&6724-StratoAG&DE&	1.1M &5.1\% \\
%         Rest& -- & -- & 5.9M & 27\% \\
%     \end{tabular}
%     \caption{Top 5 Hosting ASes for IPv6: 2021}
%     \label{tab:top5-2021-ipv6}
% \end{table}

\begin{figure}
    \centering
    \includegraphics[width=1\linewidth]{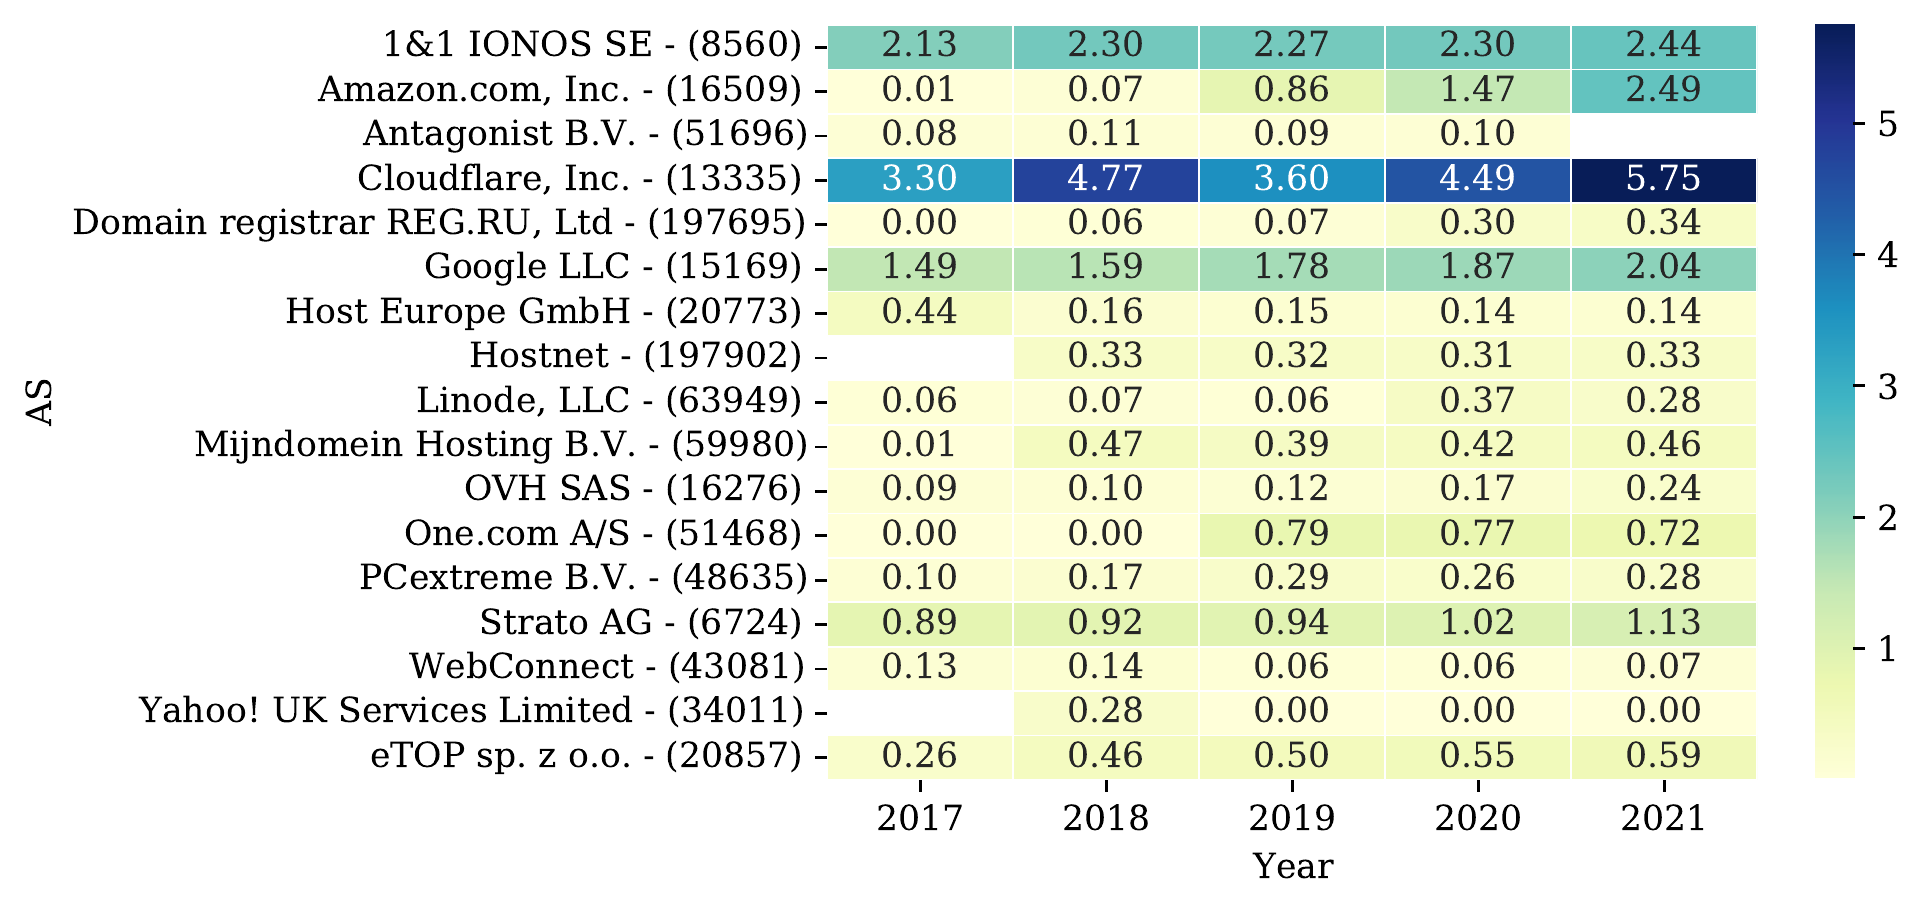}
    \caption{Top Hosting ASes  evolution (million domains IPv6)}
    \label{fig:v6-top10ASes}
\end{figure}

\autoref{tab:datasets-v6} shows the results for IPv6 (we consider AAAA~\cite{rfc3596} use instead of A records for IPv6). We see far fewer domains with IPv6 hosting.

\autoref{fig:v6-top5-time} shows the hosting concentration changes for IPv6, for the 5 top hosting ASes. 

\begin{figure}
    \centering
    \includegraphics[width=1\linewidth]{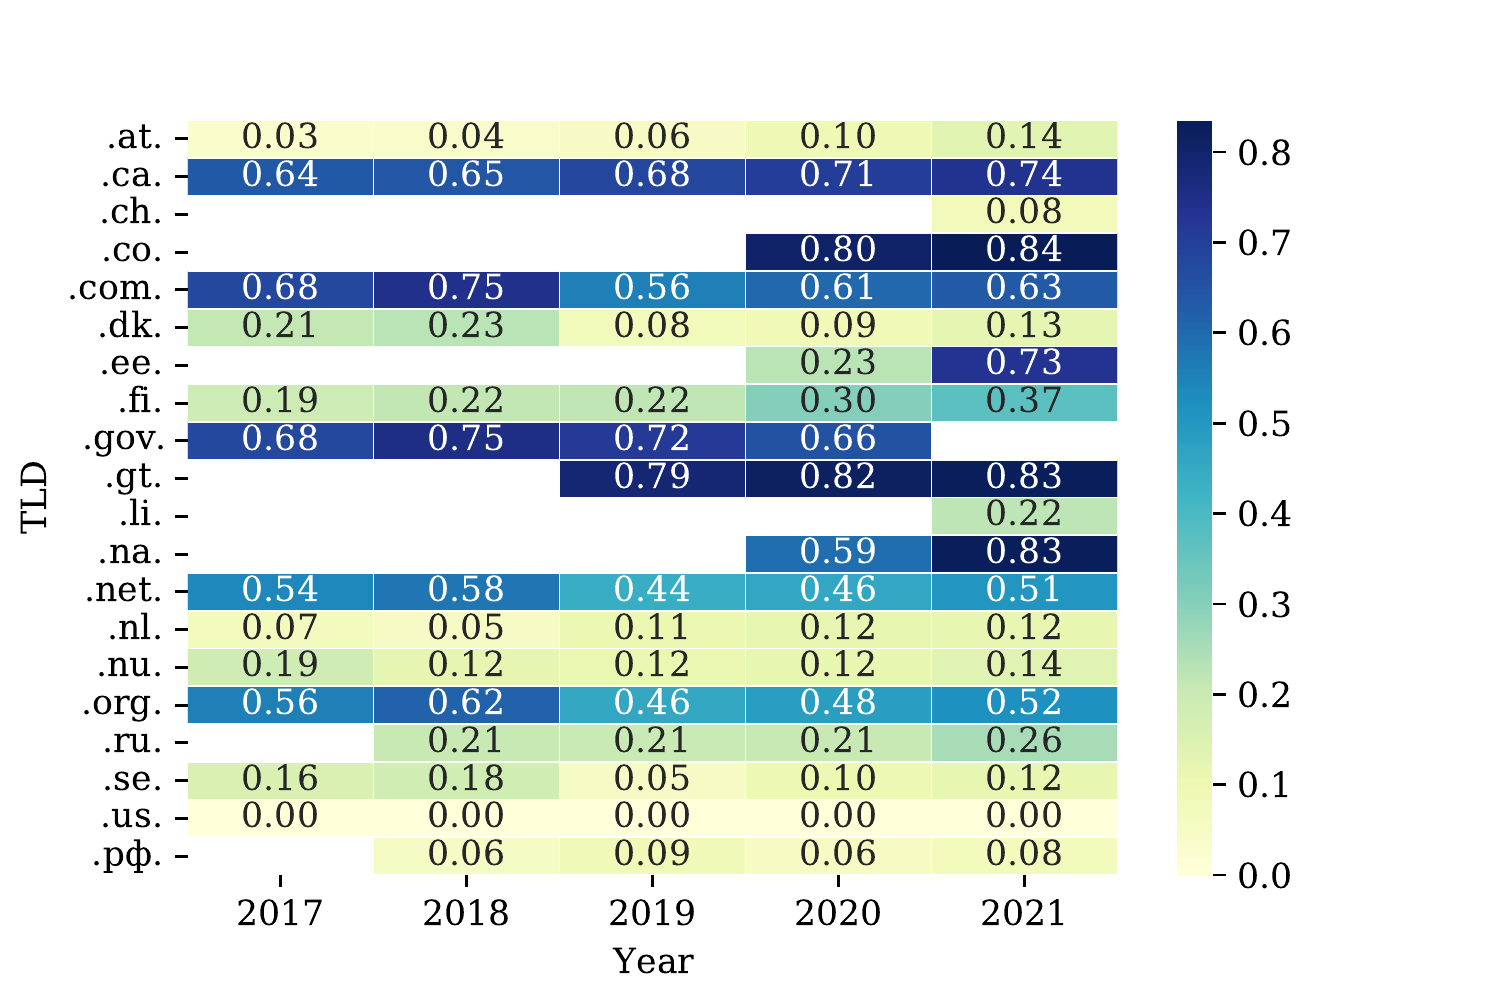}
    %  \caption{Concentration changes for Top 5 hosting ASes and TLDs
    \caption{Top 5 hosting companies  share (IPv6)}
    \label{fig:v6-top5-time}
\end{figure}

\begin{figure}
    \centering
    \includegraphics[width=1\linewidth]{res/typeOverTimev6.pdf}
    %  \caption{Concentration changes for Top 5 hosting ASes and TLDs
    \caption{Top 5 hosting companies  share (IPv6)}
    \label{fig:v6-top5-time}
\end{figure}

% \begin{figure}
%  \includegraphics[width=1\linewidth]{res/typeOverTimev6.pdf}
% %  \caption{Concentration changes for Top 5 hosting ASes and TLDs
%  \caption{Top 5 hosting companies  share (IPv6)}
% %  \label{fig:v6-top5-time}
% 
% \end{figure}

\autoref{fig:v6-type-time} shows the evolution of US hosting companies per TLD for IPv6.

\begin{figure}
    \centering
    % 
    %    \subfloat[ IPv4    \label{fig:v4-type-time}]{\includegraphics[width=.8\linewidth]{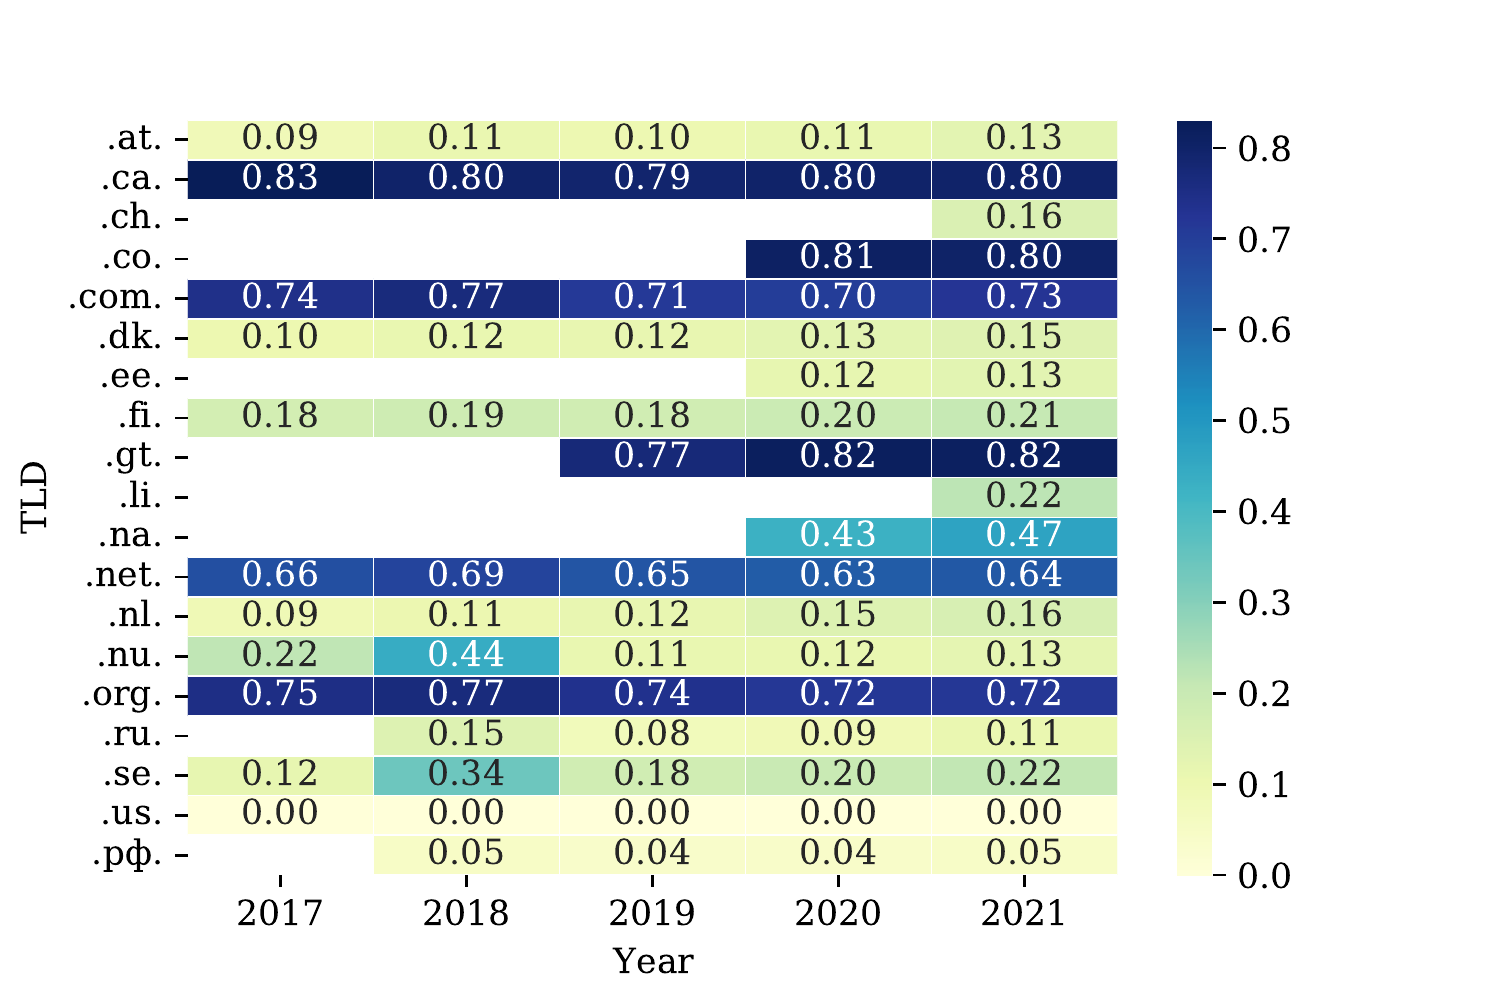}}\\
    %    \subfloat[ IPv6    \label{fig:v6-type-time}]{\includegraphics[width=.8\linewidth]{res/typeOverTimev6.pdf}}\\
    \includegraphics[width=1\linewidth]{res/typeOverTimev6.pdf}
    \caption{Evolution of US hosting presence per TLD (IPv6)}
    \label{fig:v6-type-time}
\end{figure}

% 
% 
% 
% 
% 
% \begin{figure}
% 
%    \subfloat[ IPv4    \label{fig:conc-top10-ipv4}]{\includegraphics[width=1\linewidth]{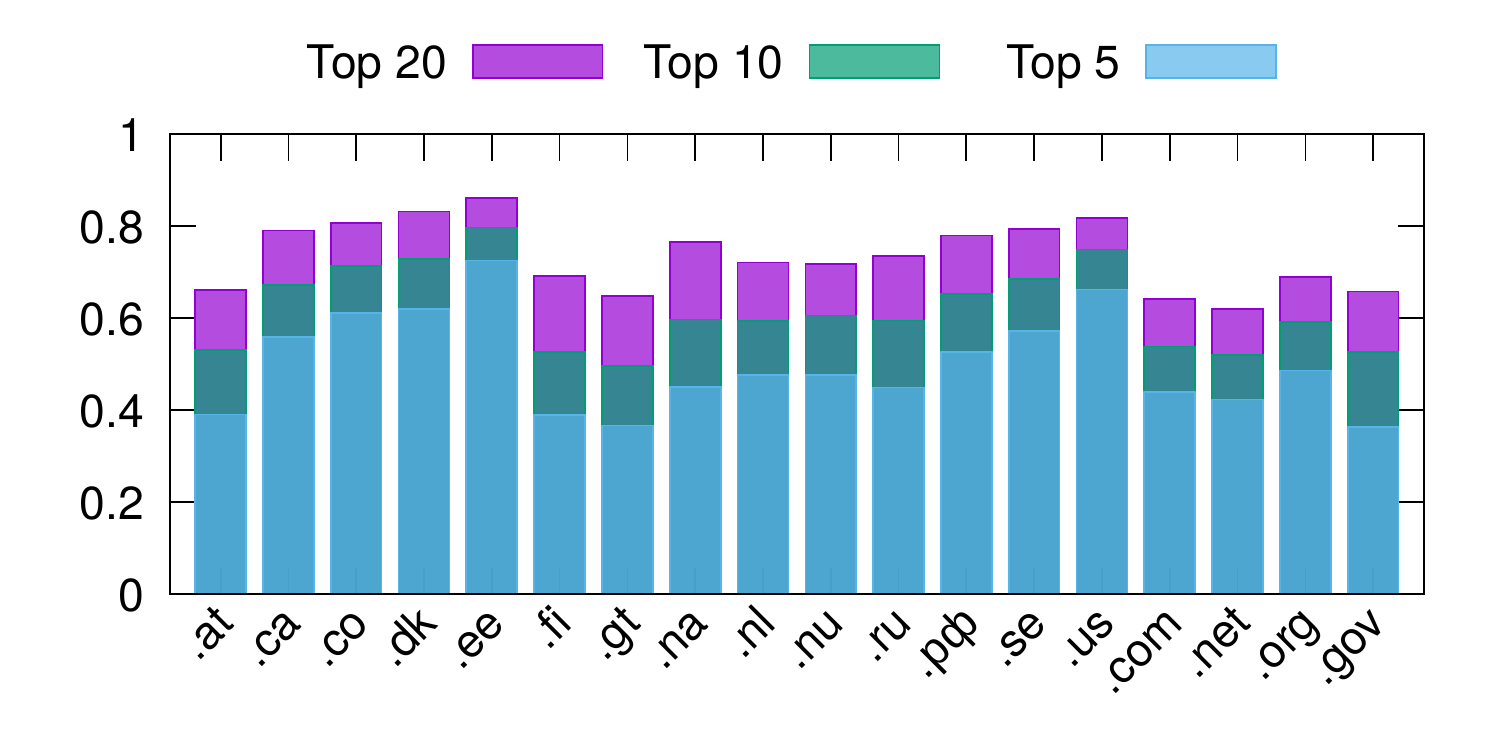}}\\
%    \subfloat[ IPv6    \label{fig:conc-top10-ipv6}]{\includegraphics[width=1\linewidth]{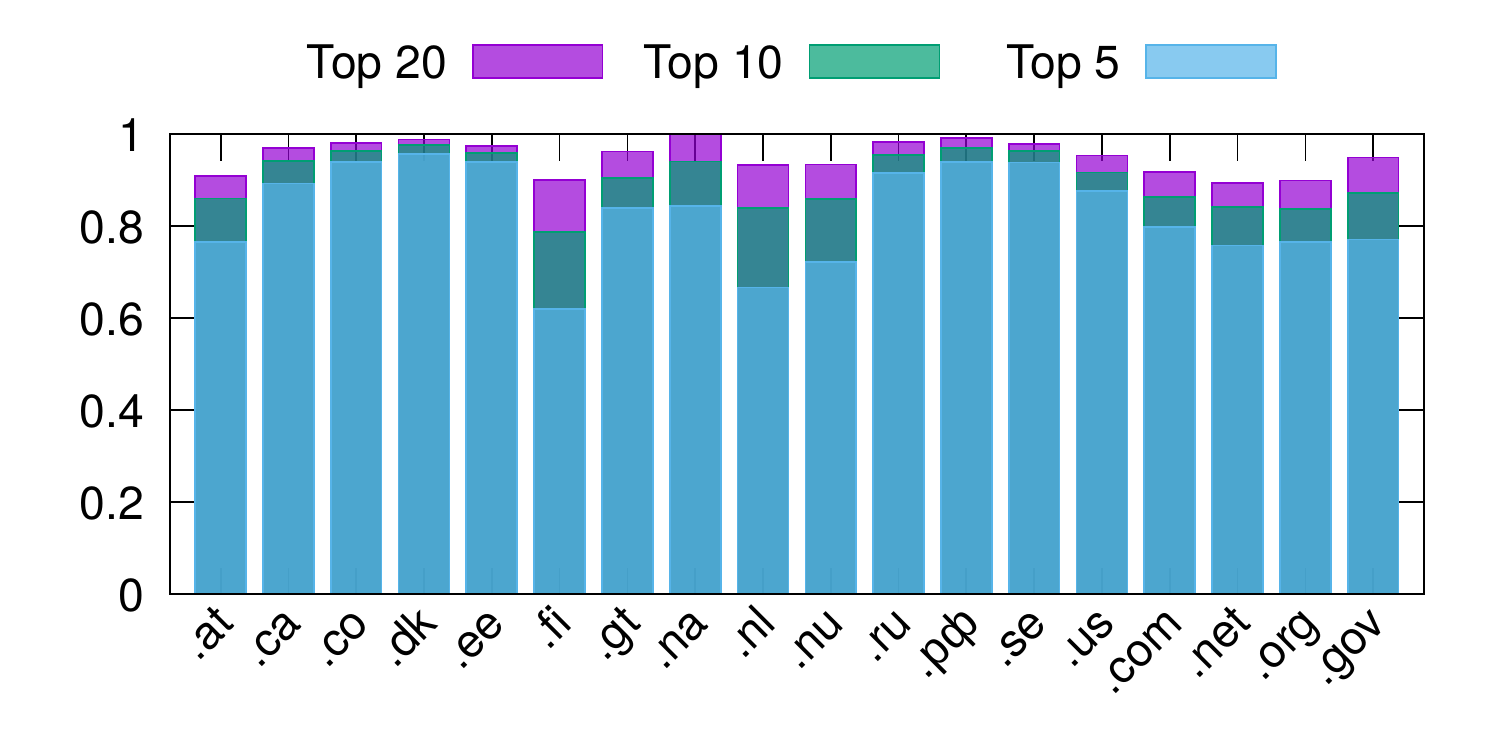}}\\
% 
%  \caption{Hosting concentration 2020}
%  
% 
% \label{fig:conc-top10-2020}
% \end{figure}
% 
% 
% 
% \begin{figure}
% 
%    \subfloat[ IPv4    \label{fig:conc-top10-ipv4}]{\includegraphics[width=1\linewidth]{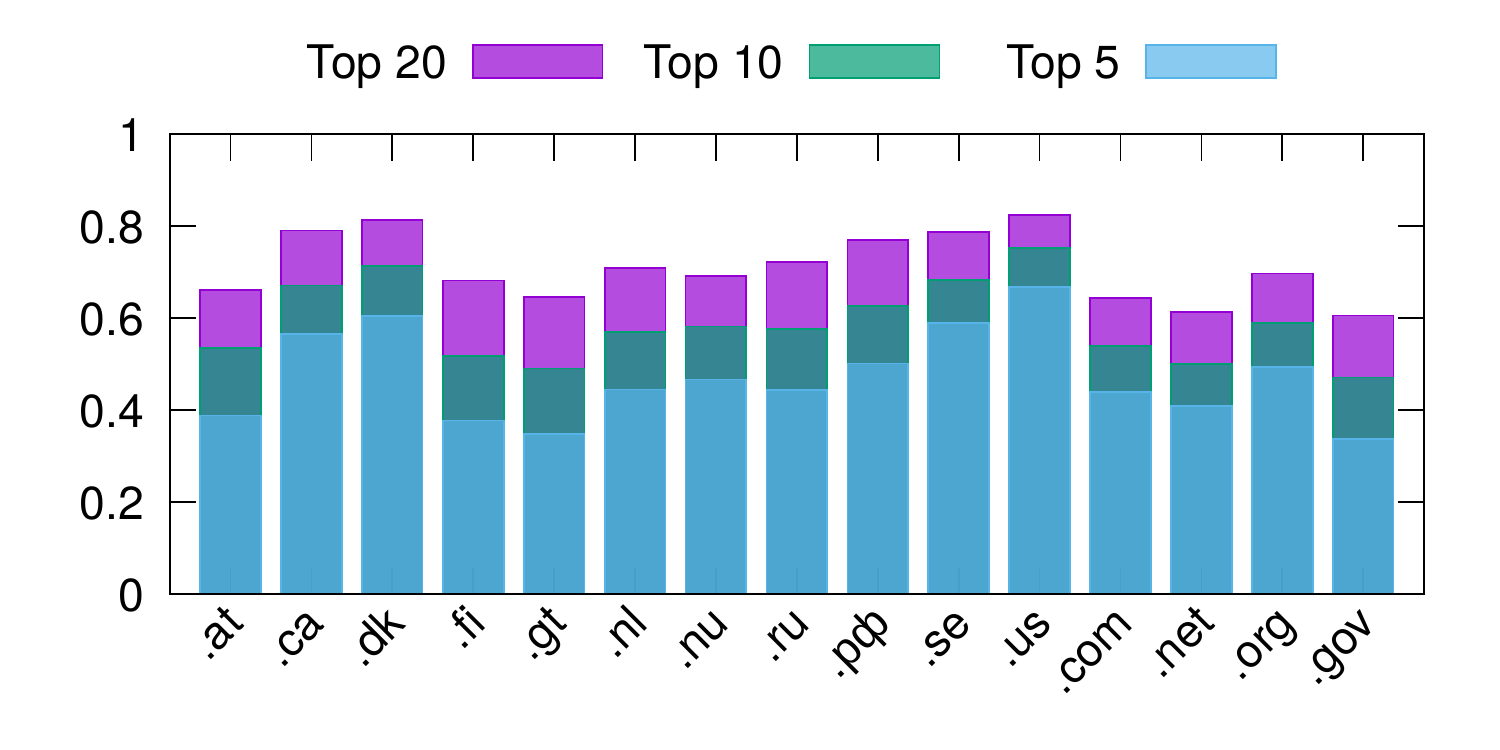}}\\
%    \subfloat[ IPv6    \label{fig:conc-top10-ipv6}]{\includegraphics[width=1\linewidth]{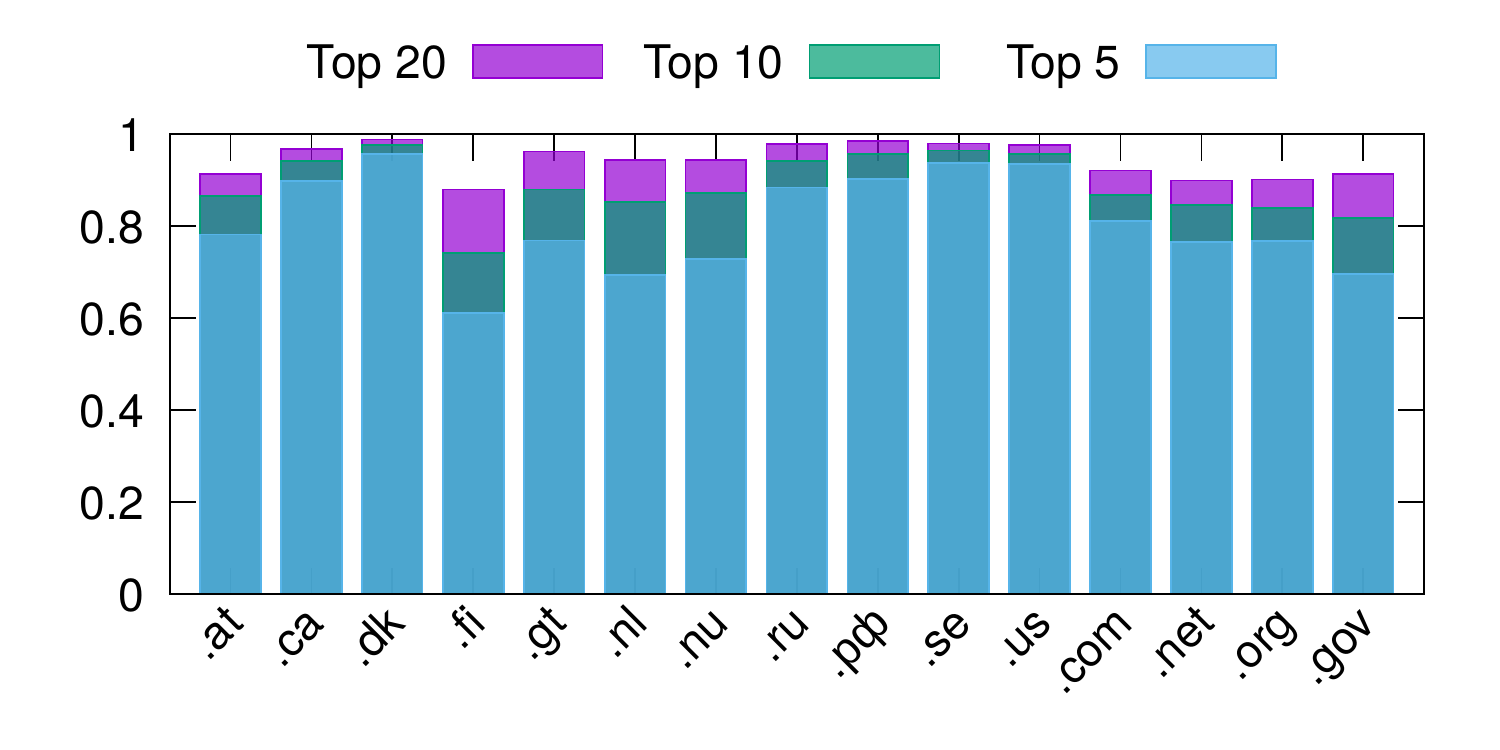}}\\
% 
%  \caption{Hosting concentration 2019}
%  
% 
% \label{fig:conc-top10-2019}
% \end{figure}
% 
% 
% 
% \begin{figure}
% 
%    \subfloat[ IPv4    \label{fig:conc-top10-ipv4}]{\includegraphics[width=1\linewidth]{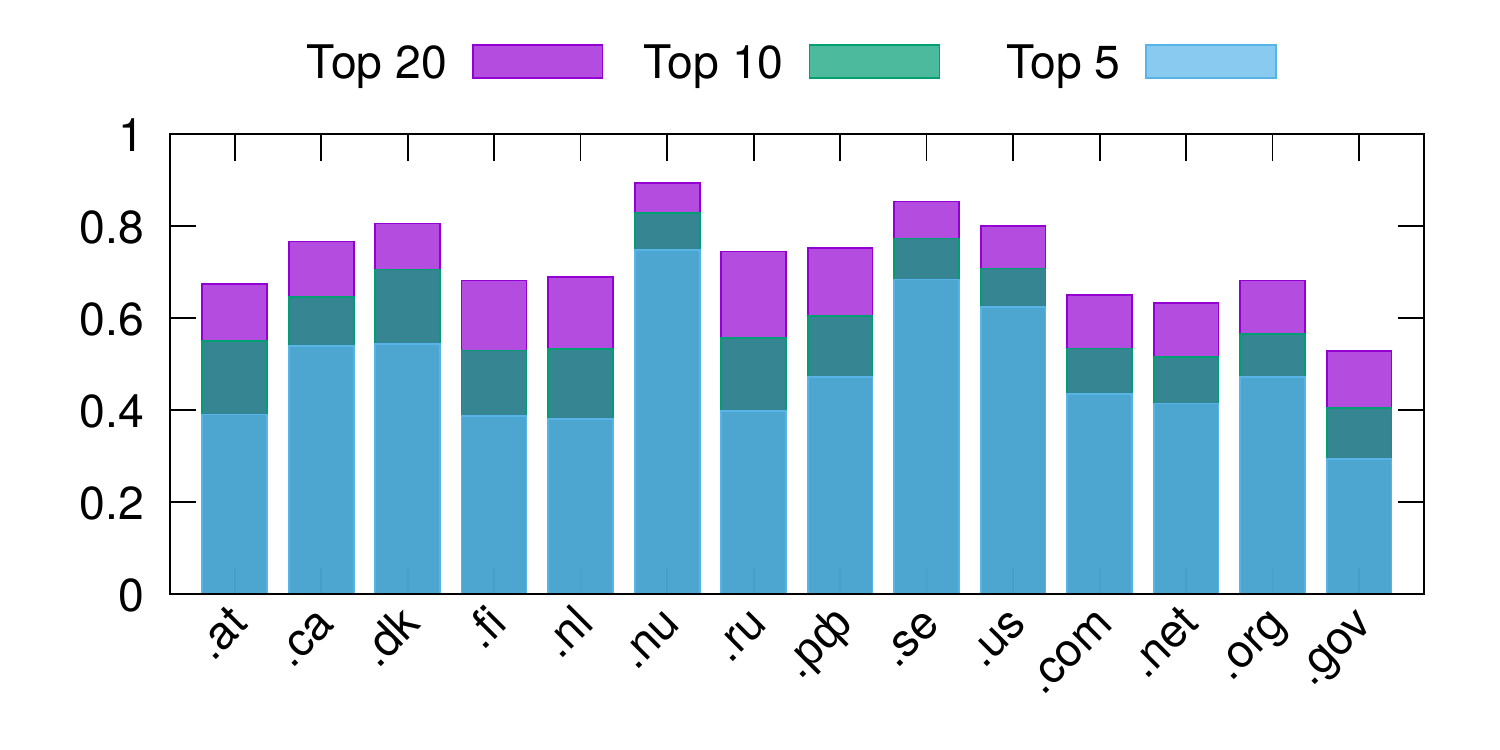}}\\
%    \subfloat[ IPv6    \label{fig:conc-top10-ipv6}]{\includegraphics[width=1\linewidth]{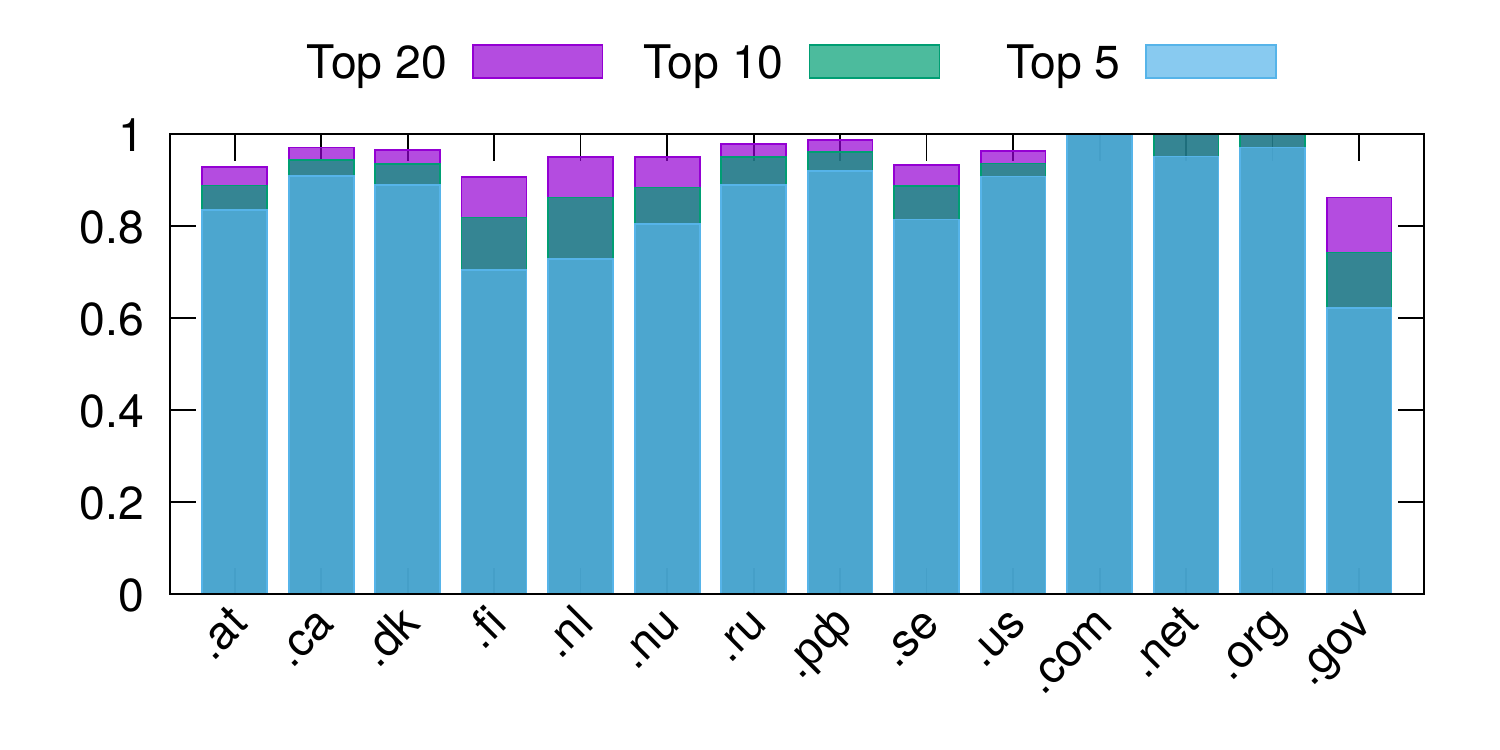}}\\
% 
%  \caption{Hosting concentration 2018}
%  
% 
% \label{fig:conc-top10-2018}
% \end{figure}
% 
% 
% 
% 
% 
% 
% 
% \begin{figure}
% 
%    \subfloat[ IPv4    \label{fig:conc-top10-ipv4}]{\includegraphics[width=1\linewidth]{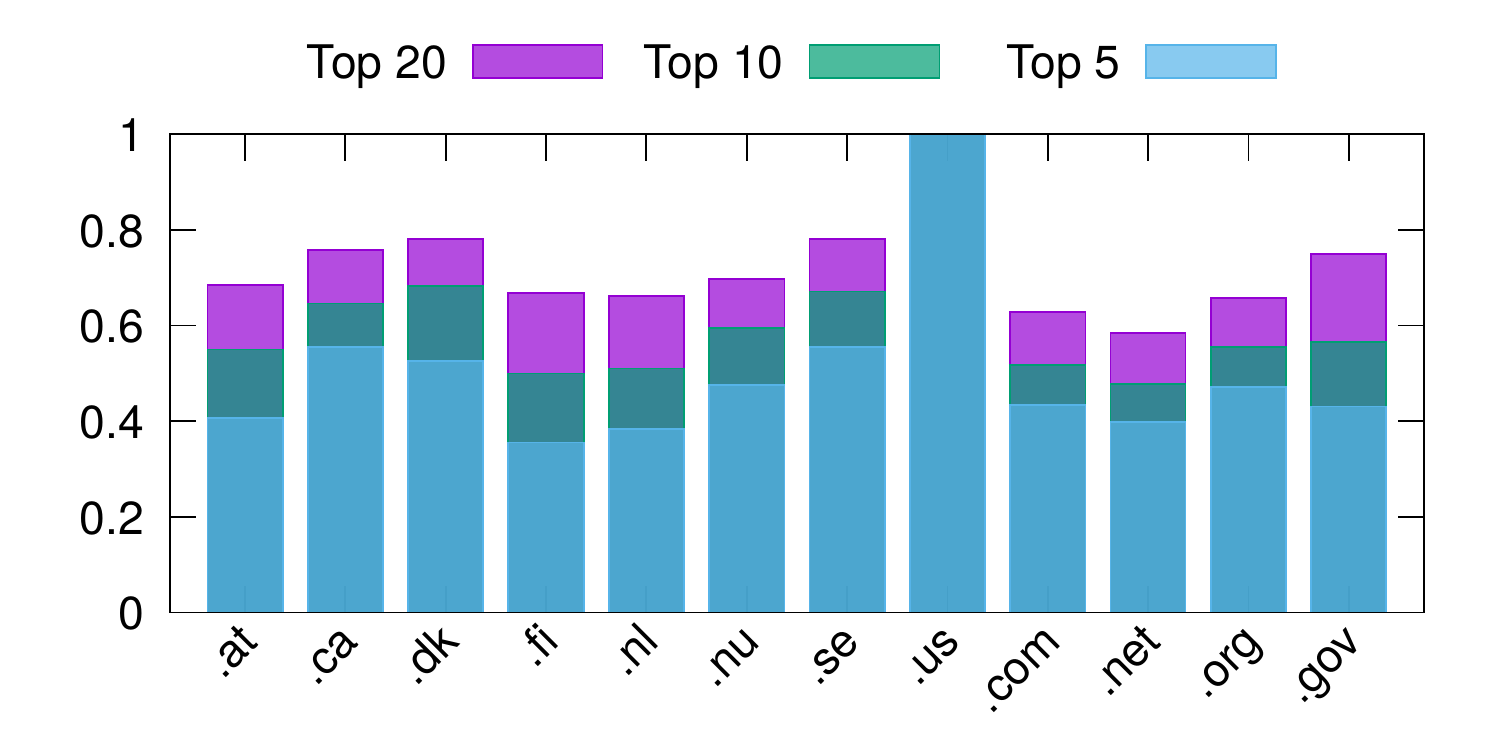}}\\
%    \subfloat[ IPv6    \label{fig:conc-top10-ipv6}]{\includegraphics[width=1\linewidth]{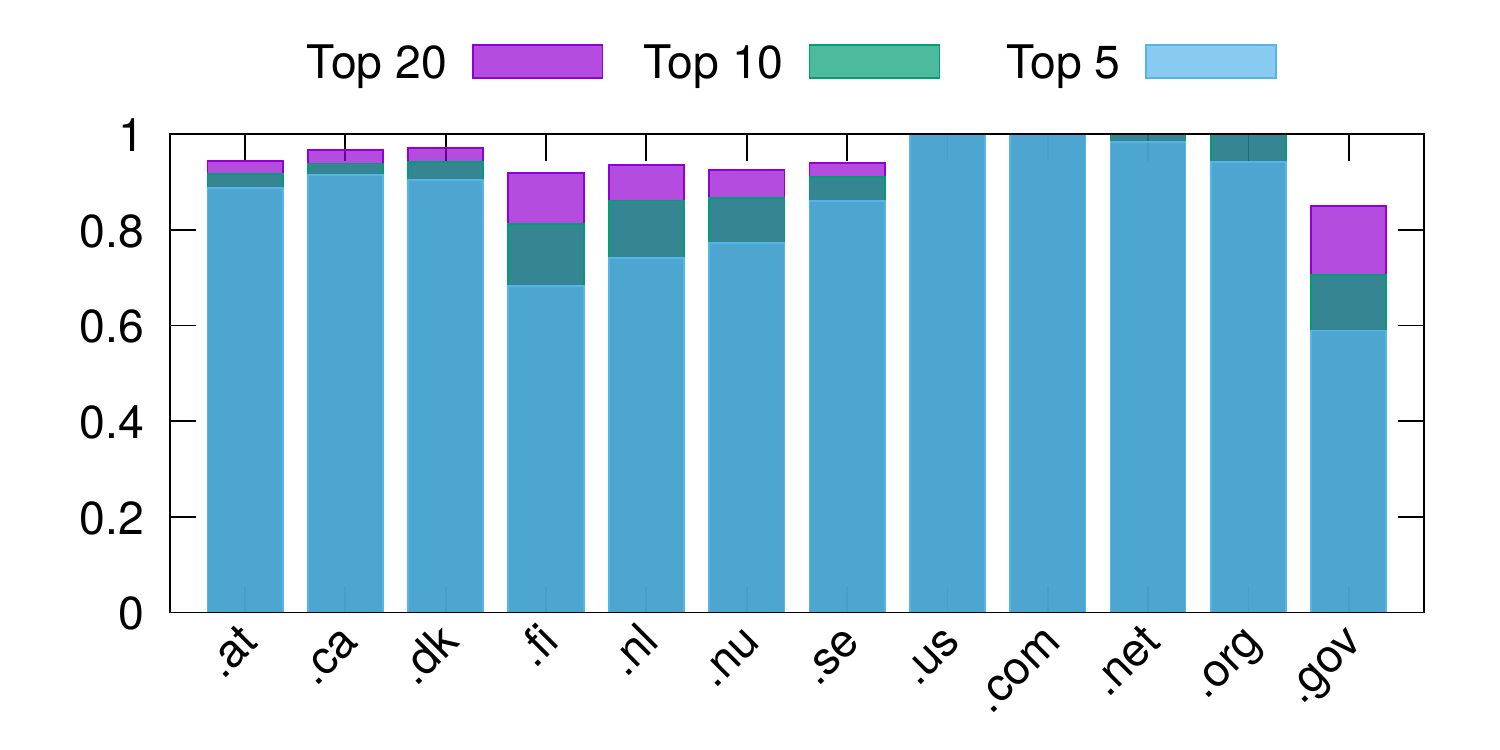}}\\
% 
%  \caption{Hosting concentration 2017}
%  
% 
% \label{fig:conc-top10-2017}
% \end{figure}
